# Supplementary material for: Hyperfine structure and electric quadrupole transitions in the deuterium molecular ion
Source: arXiv:2006.15039 ancillary file (2020-12-16)
Supplement: Supplementary file 1 [file suppl.pdf]

The supplemental material includes the following five ASCII files with tables that were only partly presented in the text of the paper:

1. `d2plus-Heff.lst` with the coefficients $E_n, n = 1, \ldots, 6$ of the effective spin Hamiltonian $H^{\rm eff}$ of $D_2^+$ in the ro-vibrational states with orbital momentum $L = 1, \ldots, 4$ and vibrational quantum number $v \leq 10$.

2. `d2plus-hfs-evnL.lst` with the hyperfine shift of the energy level $\Delta E^{(vL)IFJ}$, the mixing coefficients $\beta^{(vL)IFJ}_{I'F'}$, and the derivatives of the hyperfine shift with respect to the coefficients of the effective spin Hamiltonian $\Gamma^{(vL)IFJ}_n, n = 1, ..., 6$ and to the deuteron electric quadrupole moment, $\partial \Delta E^{(vL)IFJ}/\partial Q_d$, for states with $v \leq 10$ and *even* values of the orbital momentum $L = 0, 2, 4$.

3. `d2plus-hfs-oddL.lst` with the hyperfine shift of the energy level $\Delta E^{(vL)IFJ}$, the mixing coefficients $\beta^{(vL)IFJ}_{I'F'}$, and the derivatives of the hyperfine shift with respect to the coefficients of the effective spin Hamiltonian $\Gamma^{(vL)IFJ}_n, n = 1, ...6$ and to the deuteron electric quadrupole moment, $\partial \Delta E^{(vL)IFJ}/\partial Q_d$, for states with $v \leq 10$ and *odd* values of the orbital momentum $L = 1, 3$.

4. `d2plus-E2-evnL.lst` with the hyperfine shift of the $E2$-transition frequency $\Delta E^{\rm hfs}$, its derivatives $\Gamma_{in}$ and $\Gamma'_{in}$ with respect to the coefficients $E_n$ and $E'_n$ of the effective spin Hamiltonian of the initial and final states $(vL)$ and $(v'L')$, respectively, and the derivative with respect to $Q_d$, $\partial \Delta E^{\rm hfs}/\partial Q_d$, the relative intensity $\mathcal{W}^{\rm hfs} = \mathcal{W}^{\rm hfs}((v'L')IFJ'; (vL)IFJ)$ of the strong (favored) hyperfine components of the $E2$-transition lines between states with $v \leq 10$ and *even* values $L \leq 4$.

5. `d2plus-E2-oddL.lst` with the hyperfine shift of the $E2$-transition frequency $\Delta E^{\rm hfs}$, its derivatives $\Gamma_{in}$ and $\Gamma'_{in}$ with respect to the coefficients $E_n$ and $E'_n$ of the effective spin Hamiltonian of the initial and final states $(vL)$ and $(v'L')$, respectively, and the derivative with respect to $Q_d$, $\partial \Delta E^{\rm hfs}/\partial Q_d$, the relative intensity $\mathcal{W}^{\rm hfs} = \mathcal{W}^{\rm hfs}((v'L')IFJ'; (vL)IFJ)$ of the strong (favored) hyperfine components of the $E2$-transition lines between states with $v \leq 10$ and *odd* values $L = 1, 3$.

The above ASCII files contain uniformly formatted lines without any special symbols. The data in each line are separated by one or more spaces and appear in the order described below.

1. `d2plus-Heff.lst`

The file contains 55 lines. In each line are given the quantum numbers $v$ and $L$ (integers), and the six coefficients $E_n, n = 1, \ldots, 6$ in units of MHz.

2. `d2plus-hfs-evnL.lst`

Each of the 286 lines contains the description of one hyperfine component, as follows:
– the ordinal number of the line;
– the quantum numbers $v$ and $L$ (integers);
– the quantum numbers of the hyperfine component $I$, $F$, and $J$ (printed as real numbers);
– the hyperfine shift $\Delta E^{(vL)IFJ}/h$ of the energy level, in MHz;
– the uncertainty $u(\Delta E^{(vL)IFJ}/h)$ of the hyperfine shift $\Delta E^{(vL)IFJ}/h$, in kHz;
– the five expansion coefficients $\beta^{(vL)IFJ}_{0,1/2}$, $\beta^{(vL)IFJ}_{1,1/2}$, $\beta^{(vL)IFJ}_{1,3/2}$, $\beta^{(vL)IFJ}_{2,3/2}$, $\beta^{(vL)IFJ}_{2,5/2}$;
– the derivatives $\Gamma^{(vL)IFJ}_n, n = 1, ..., 6$, in MHz;
– the derivative $d\Delta E^{(vL)IFJ}/dQ_d$, in kHz fm$^{-2}$.

3. `d2plus-hfs-oddL.lst`

Same as `d2plus-hfs-evnL.lst`, for states with *odd* $L$, with a total of 121 lines.

4. `d2plus-E2-evnL.lst`

For each allowed $E2$ transition $(vL) \to (v'L')$ between rovibrational states with $v, v' \leq 10$ and *even* values of the orbital momentum $L, L' \leq 4$, are given:

- a title line with the non-relativistic quantum numbers of the initial and final states in the form " ( v,L)−> ( v'L')" ;

- the characteristics of the strong (favored) hyperfine components $|(vL)IFJ\rangle \to |(v'L')IFJ'\rangle$ in increasing order of the hyperfine shift $\Delta E^{\rm hfs} = \Delta E^{(v'L')IFJ'} - \Delta E^{(vL)IFJ}$, one data line for each favored component. Each data line includes:
  – the ordinal number $i$ of the favored hyperfine component;

– the quantum numbers $I$ (integer), and $F$, $J$, $J'$ (real);
– the hyperfine shift of the $E2$-transition frequency $\Delta E^{\rm hfs}/h = (\Delta E^{(v'L')IFJ'} - \Delta E^{(vL)IFJ})/h$, in MHz;
– the uncertainty $u(\Delta E^{\rm hfs})/h$ of the hyperfine shift $\Delta E^{\rm hfs}$, in kHz;
– the relative intensity $\mathcal{W}^{\rm hfs}((v'L')IFJ';(vL)IFJ)$;
– the six derivatives $\Gamma'_{in} = E'_n(\partial\Delta E^{\rm hfs}/\partial E'_n), n = 1,...,6$ with respect to the coefficients $E'_n$ of the effective spin Hamiltonian of the final state $(v'L')$;
– the six derivatives $\Gamma_{in} = E_n(\partial\Delta E^{\rm hfs}/\partial E_n), n = 1,...,6$ with respect to the coefficients $E_n$ of the effective spin Hamiltonian of the initial state $(vL)$;
– the derivative $d\Delta E^{\rm hfs}/dQ_d$, in kHz fm$^{-2}$.

5. `d2plus-E2-oddL.lst`
Same as `d2plus-E2-evnL.lst`, but for the allowed $E2$ transitions between rovibrational states with $v, v' \leq 10$ and *odd* values $L, L' = 1, 3$.
